# Supplementary material for: Comparison of Information-Gain Criteria for Action Selection
Source: arXiv:2109.13540 source file (2022-05-07)
Supplement: Supplementary file 1 [file appendix.tex]

\appendices
\label{sec:appendix}
\section{Mathematical Notation}
The mathematical notation and formulations used in the paper is detailed below:
\begin{itemize}
    \item Let ${}^A H_B \in \mathbb{R}^{4 \times 4}$ be the homogeneous transformation matrix describing the transformation of a point from the frame B to the frame A. ${}^A H_B = \begin{bmatrix} {}^A \mathbf{R}_B & {}^A \mathbf{t}_B \\  0_{1\times 3} & 1 \end{bmatrix}$ where ${}^A R_B$ is the rotation matrix and ${}^A o_B$ is the translation vector of frame B with respect to frame A.
    \item Let $\widetilde{\mathbf{q}}$ denote a general quaternion, where $\mathbf{q}$ refers to the vector component of the quaternion and $q_0$ to the real part such that $\widetilde{\mathbf{q}} = [q_{0}, \mathbf{q}^T]^T$. Basic operations on quaternions is defined as follows:
    \begin{itemize}
        \item A point $a \in \mathbb{R}^3$ can be represented as a quaternion $\tilde{a} = \begin{bmatrix} 0 \\ a \end{bmatrix}^T \in \mathbb{R}^4$.
        \item Scalar multiplication with a quaternion is given by: $s \widetilde{\mathbf{q}} = [s q_{0}, s\mathbf{q}^T]^T$.
        \item Addition of two quaternions is given by: $\widetilde{\mathbf{q}}_1 + \widetilde{\mathbf{q}}_2 = [q_{0_1} + q_{0_2}, (\mathbf{q}_1 + \mathbf{q}_2)^T]^T$.
        \item Multiplication of two quaternions is given by: 
        \begin{equation}
        \begin{aligned}
            \widetilde{\mathbf{q}}_1 \odot \widetilde{\mathbf{q}}_2  
            &= \begin{bmatrix}
            q_{0_1} & -\mathbf{q_1}^T \\ \mathbf{q_1} & \mathbf{q_1}^{\times} + q_{0_1}\mathbb{I}_3  
            \end{bmatrix}\widetilde{\mathbf{q}}_2 \quad , \\
            &= \begin{bmatrix}
            q_{0_2} & -\mathbf{q_2}^T \\ \mathbf{q_2} & -\mathbf{q_2}^{\times} + q_{0_2}\mathbb{I}_3  
            \end{bmatrix}\widetilde{\mathbf{q}}_1 \quad ,
        \end{aligned}
        \label{eq:quaternionmult}
        \end{equation}
        where $\odot$ is the quaternion multiplication operator and $[v]^{\times}$ is the skew-symmetric matrix formed from the vector $v$.
        \item Conjugate $\widetilde{\mathbf{q}}^{*}$ is given by $\widetilde{\mathbf{q}}^{*} = [q_0, -\mathbf{q^T}]$.
        \item The norm of a quaternion is $||\widetilde{\mathbf{q}}|| = \sqrt{\widetilde{\mathbf{q}}\odot \widetilde{\mathbf{q}}^*}$ and a unit quaternion is one with $||\widetilde{\mathbf{q}}|| = 1$.
    \end{itemize}
\end{itemize}
